# Supplementary material for: Identifying Actionable Messages on Social Media
Source: arXiv:1511.00722 source file (2015-11-02)
Supplement: Supplementary file 1 [file actionability_appendix.tex]

\begin{figure*}
\centering

\begin{subfigure}[b]{0.48\textwidth}
  \centering
  \includegraphics[width=0.95\textwidth]{figure/eps/full_spec_vs_best_eval/network_f1_regular_namespace_vs_best_namespace}
  \caption{Network original namespace vs best namespace}
  \label{fig:network_f1_regular_namespace_vs_best_namespace}
\end{subfigure}
\begin{subfigure}[b]{0.48\textwidth}
  \centering
  \includegraphics[width=0.95\textwidth]{figure/eps/full_spec_vs_best_eval/network_f1_best_namespace_vs_best_model_namespace}
  \caption{Network best namespace vs model, namespace}
  \label{fig:network_f1_best_namespace_vs_best_model_namespace}
\end{subfigure}

\caption{F1}
\label{fig:f1_scatter}
\end{figure*}

This is the graveyard for the unused content.

This is now just place holder

\begin{figure*}
\centering
\begin{subfigure}[b]{0.32\textwidth}
  \centering
  \includegraphics[width=0.95\textwidth]{figure/eps/model_by_type_prec_rec/model_by_type_prec_rec}
  \caption{Different model types}
  \label{fig:model_by_type_prec_rec}
\end{subfigure}
\begin{subfigure}[b]{0.32\textwidth}
  \centering
  \includegraphics[width=0.95\textwidth]{figure/eps/model_by_type_prec_rec/model_by_type_prec_rec_full_spec_model}
  \caption{Fully specified COMPANY-LANGUAGE-SOURCE model}
  \label{fig:model_by_type_prec_rec_full_spec_model}
\end{subfigure}
\begin{subfigure}[b]{0.32\textwidth}
  \centering
  \includegraphics[width=0.95\textwidth]{figure/eps/model_by_type_prec_rec/model_by_type_prec_rec_genric_model}
  \caption{Fully generic *-*-* model}
  \label{fig:model_by_type_prec_rec_genric_model}
\end{subfigure}
\caption{F1}
\label{fig:various_scatter}
\end{figure*}

\begin{figure*}
\centering

\begin{subfigure}[b]{0.48\textwidth}
  \centering
  \includegraphics[width=0.95\textwidth]{figure/eps/full_spec_vs_best_eval/language_f1_best_namespace_vs_best_model_namespace}
  \caption{Language best namespace vs model, namespace}
  \label{fig:language_f1_best_namespace_vs_best_model_namespace}
\end{subfigure}
\begin{subfigure}[b]{0.48\textwidth}
  \centering
  \includegraphics[width=0.95\textwidth]{figure/eps/full_spec_vs_best_eval/language_f1_regular_namespace_vs_best_namespace}
  \caption{Language original namespace vs best namespace}
  \label{fig:language_f1_regular_namespace_vs_best_namespace}
\end{subfigure}

\begin{subfigure}[b]{0.48\textwidth}
  \centering
  \includegraphics[width=0.95\textwidth]{figure/eps/full_spec_vs_best_eval/company_f1_best_namespace_vs_best_model_namespace.eps}
  \caption{Company best namespace vs model, namespace}
  \label{fig:company_f1_best_namespace_vs_best_model_namespace}
\end{subfigure}
\begin{subfigure}[b]{0.48\textwidth}
  \centering
  \includegraphics[width=0.95\textwidth]{figure/eps/full_spec_vs_best_eval/company_f1_regular_namespace_vs_best_namespace.eps}
  \caption{Company original namespace vs best namespace}
  \label{fig:company_f1_regular_namespace_vs_best_namespace}
\end{subfigure}

\caption{F1}
\label{fig:f1_scatter}
\end{figure*}
